# Supplementary material for: MaskGIT: Masked Generative Image Transformer
Source: arXiv:2202.04200 source file (2022-02-08)
Supplement: Supplementary file 1 [file supp1_class_cond_diversity.tex]

\newcommand{\tmpwidth}{0.33\linewidth}

\begin{figure*}[!ht]
    \centering
    \begin{tabular}{c c c c}

    \includegraphics[ width=\tmpwidth]{figures/diversity/130_biggan_trun1.png} & \hspace{-3mm}
    \includegraphics[ width=\tmpwidth]{figures/diversity/130_ours.png} & \hspace{-3mm}
    \includegraphics[ width=\tmpwidth]{figures/diversity/130_gt.png} \\ 
    
    \includegraphics[ width=\tmpwidth]{figures/diversity/145_biggan_trun1.png} & \hspace{-3mm}
    \includegraphics[ width=\tmpwidth]{figures/diversity/145_ours.png} & \hspace{-3mm}
    \includegraphics[ width=\tmpwidth]{figures/diversity/145_gt.png} \\
    
    \includegraphics[ width=\tmpwidth]{figures/diversity/000_biggan_trun1.png} & \hspace{-3mm}
    \includegraphics[ width=\tmpwidth]{figures/diversity/000_ours1.png} & \hspace{-3mm}
    \includegraphics[ width=\tmpwidth]{figures/diversity/000_gt.png} \\   
    
    BigGAN-deep (FID=$6.95$) & \model (FID=\bestfid) & Training Set \\
    \end{tabular}
    \caption{More Sample Diversity Comparisons for BigGAN-deep with truncation $1.0$ and our proposed method \model on ImageNet.}
    % \vspace{-6mm}
    \label{fig:supp_diversity}
\end{figure*}
